# Supplementary material for: Theoretical Investigations of Electronic Structure, Magnetic and Optical Properties of Transition Metal-dinuclear Molecules
Source: arXiv:1912.08586 source file (2019-12-18)
Supplement: Supplementary file 1 [file SI.pdf]

# Theoretical Investigations of Electronic Structure, Magnetic and Optical Properties of Transition Metal-dinuclear Molecules

*Indukuru Ramesh Reddy, and Kartick Tarafder**

Department of Physics, National Institute of Technology Karnataka (NITK)-Surathkal, Srinivasnagar- 575 025, Karnataka, India

The plane wave basis set and pseudo-potentials as implemented in the Vienna Ab-initio Simulation Package (VASP) was used in the GGA+U calculations[1]. The GGA+U formalism implemented via Dudarev et al.'s approach[2,3]. We varied the U values for TM atoms from 2 eV to 6 eV in order to check the consistency of U values in our calculations. We observed that the magnetic moment only on Mn atom significantly changes with different U values (See Table S1.). The results reported in the main text are for the choice of U being 6 eV at the Mn atom and 4 eV at the remaining TM atoms, and the J value set to 1 eV for all the TM atoms[4]. The distortion parameter ($\tau_4$) in the tera-coordinated geometry of the molecules was calculated using the equation $\tau_4 = (360^0-(\theta+\Phi))/141^0$, where θ (O-TM-C) and Φ (N1-TM-N2 )are the two largest angles in the tetra-coordinated geometry. The θ and Φ values are given in Table S3.

**List of Figures:**


| S. No. | Figure | Caption |
|---|---|---|
| 1 | Figure S1 | Calculated vibrational spectra of the modelled TM-dinuclear molecules |
| 2 | Figure S2 | Calculated frontier orbitals for the electronic transitions observed in Cr-dinculear molecule. (a) and (b) are the α and β orbitals, respectively. |
| 3 | Figure S3 | Calculated frontier orbitals for the electronic transitions observed in Mn-dinculear molecule. (a) and (b) are the α and β orbitals, respectively. |
| 4 | Figure S4 | Calculated frontier orbitals for the electronic transitions observed in Fe-dinculear molecule. (a) and (b) are the α and β orbitals, respectively. |
| 5 | Figure S5 | Calculated frontier orbitals for the electronic transitions observed in Co-dinculear molecule. (a) and (b) are the α and β orbitals, respectively. |
| 6 | Figure S6 | Calculated frontier orbitals for the electronic transitions observed in Cr-dinculear molecule. (a) and (b) are the α and β orbitals, respectively. |


**List of Tables:**


| S. No. | Table | Caption |
|---|---|---|
| 1 | Table S1 | Ab-initio calculated magnetic moment on TM atoms in the modelled TM-dinculear molecules with different U values. |
| 2 | Table S2 | Table S2. The calculated TM - Ligand (in Å) in the geometry of tetra-coordinated TM for the modelled TM-dinuclear molecules. |
| 3 | Table S3 | The calculated θ (O-TM-C) and Φ (N1-TM-N2) angles of the tetra-coordinated TM in the moedelled TM-dinuclear molecules. |
| 4 | Table S4 | The electronic transitions of Cr-dinuclear molecule calculated by the TD-DFT calculations, based on the optimized structure by using B3LYP functional (The corresponding molecular orbitals are shown in Figure S3). |
| 5 | Table S5 | The electronic transitions of Mn-dinuclear molecule calculated by the TD-DFT calculations, based on the optimized structure by using B3LYP functional (The corresponding molecular orbitals are shown in Figure S4). |

| | | |
|---|---|---|
| 6 | Table S6 | The electronic transitions of Fe-dinuclear molecule calculated by the TD-DFT calculations, based on the optimized structure by using B3LYP functional (The corresponding molecular orbitals are shown in Figure S5). |
| 7 | Table S7 | The electronic transitions of Co-dinuclear molecule calculated by the TD-DFT calculations, based on the optimized structure by using B3LYP functional (The corresponding molecular orbitals are shown in Figure S6). |
| 8 | Table S8 | The electronic transitions of Ni-dinuclear molecule calculated by the TD-DFT calculations, based on the optimized structure by using B3LYP functional (The corresponding molecular orbitals are shown in Figure S7). |

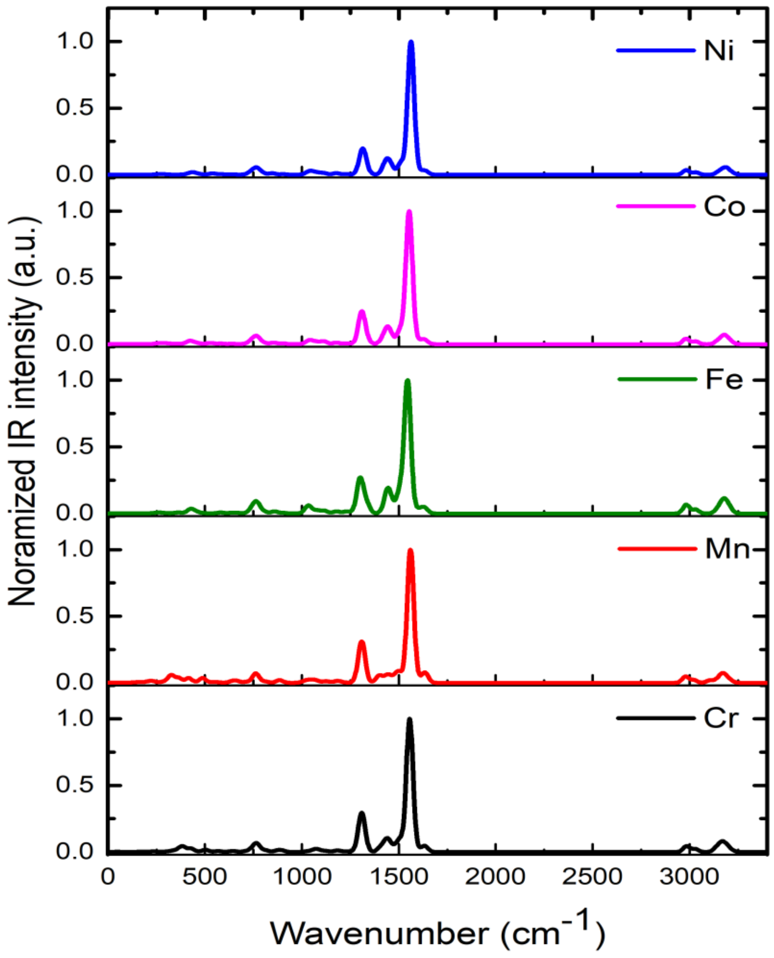


**Figure S1:** Calculated vibrational spectra of the modelled TM-dinuclear molecules

**(a)**

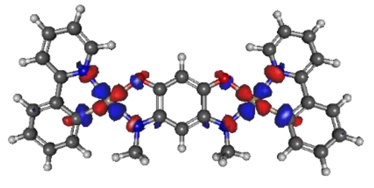
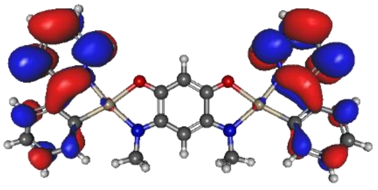
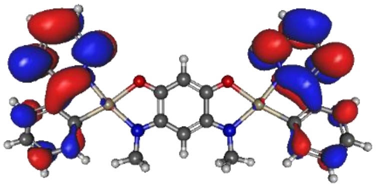

(LUMO+5) -0.0253 eV (LUMO+4) -1.1943 eV (LUMO+3) -1.1962 eV

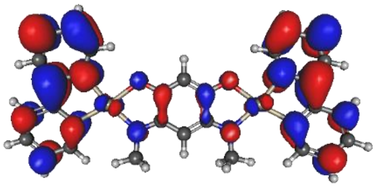
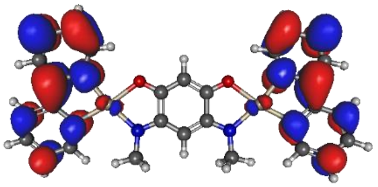
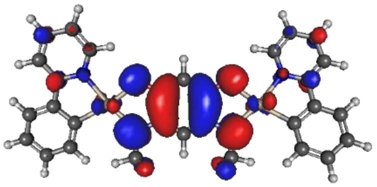

(LUMO+2) -1.6294 eV (LUMO+1) -1.6949 eV (LUMO) -2.4838 eV

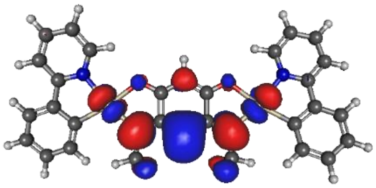
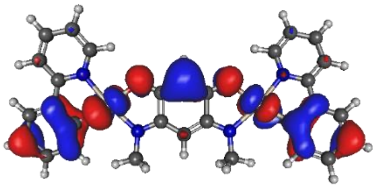
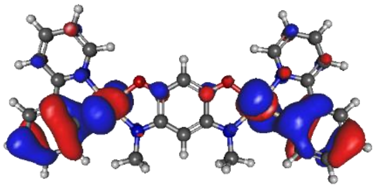

(HOMO) -5.0156 eV (HOMO-1) -5.4343 eV (HOMO-2) -5.7405 eV

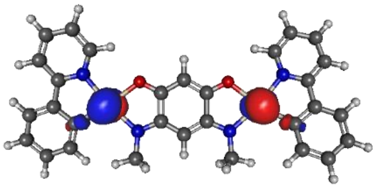
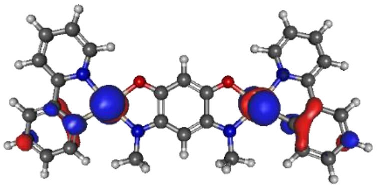
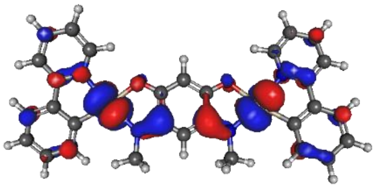

(HOMO-3) -5.7641 eV (HOMO-4) -5.7728 eV (HOMO-5) -6.0901 eV

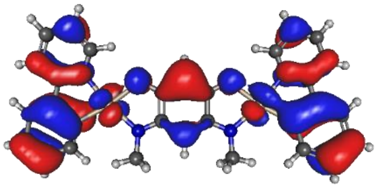

(HOMO-6) -6.1497 eV

(Continued)

**(b)**

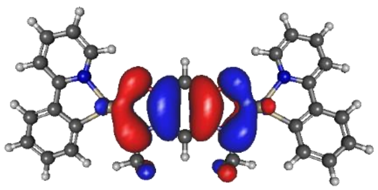

(LUMO) -2.5831 eV

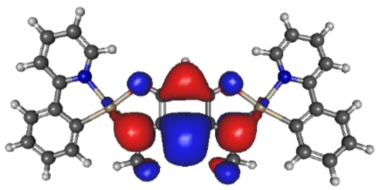

(HOMO) -5.4545 eV

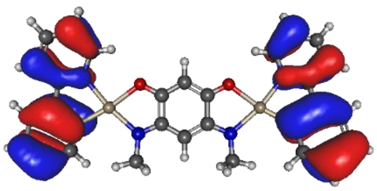

(HOMO-1) -6.2235 eV

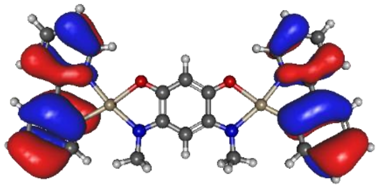

(HOMO-2) -6.2237 eV

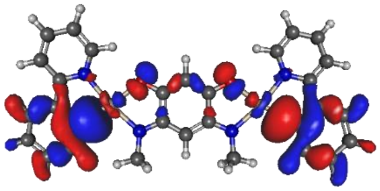

(HOMO-3) -6.3364 eV

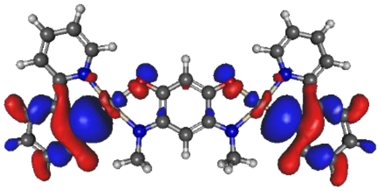

(HOMO-4) -6.3769 eV

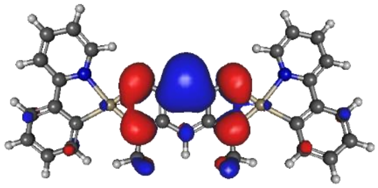

(HOMO-5) -6.4812 eV

**Figure S2:** Calculated frontier orbitals for the electronic transitions observed in Cr-dinculear molecule. (a) and (b) are the α and β orbitals, respectively.

**(a)**

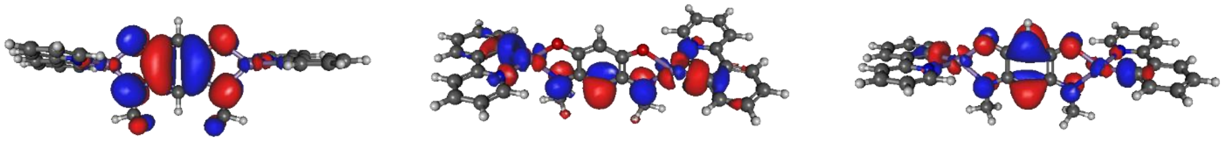

(LUMO) -2.3097 eV (HOMO) -5.0776 eV (HOMO-1) -5.436 eV

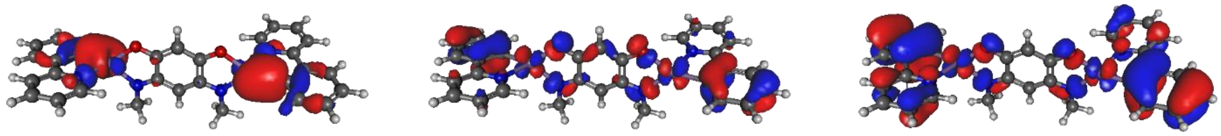

(HOMO-2) -5.4586 eV (HOMO-3) -5.935 eV (HOMO-4) -6.0447 eV

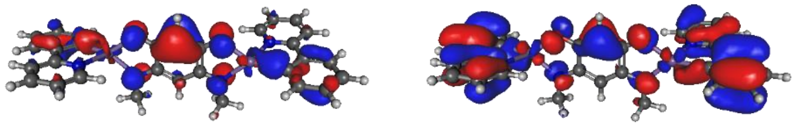

(HOMO-5) -6.3105 eV (HOMO-6) -6.3647 eV

**(b)**

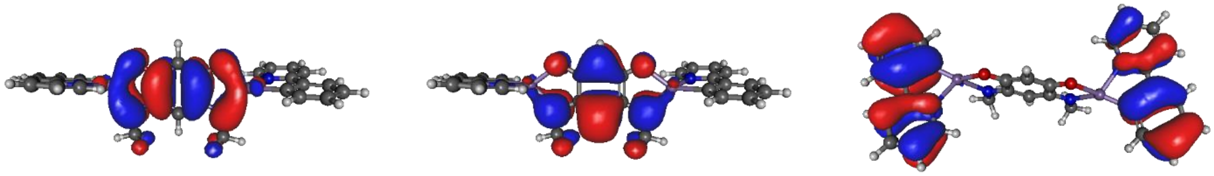

(LUMO) -2.5233 eV (HOMO) -5.393 eV (HOMO-1) -6.2578 eV

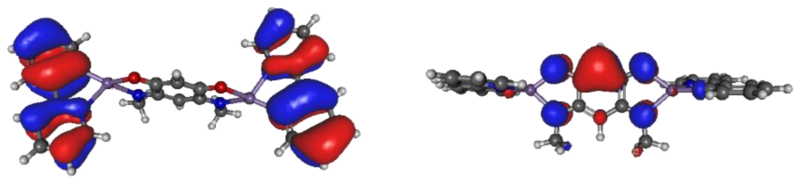

(HOMO-2) -6.2583 eV (HOMO-3) -6.3152 eV

**Figure S3:** Calculated frontier orbitals for the electronic transitions observed in Mn-dinculear molecule. (a) and (b) are the α and β orbitals, respectively.

**(a)**

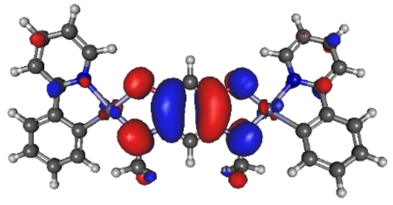

(LUMO) -2.5088 eV

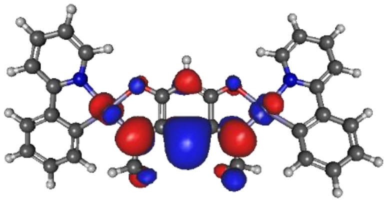

(HOMO) -5.159 eV

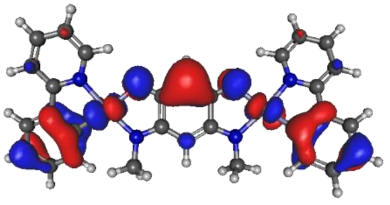

(HOMO-1) -5.7519 eV

**(b)**

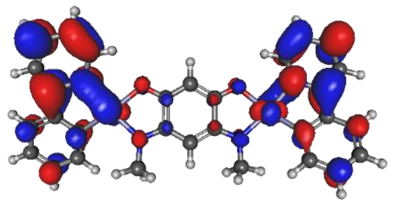

(LUMO+2) -1.7401 eV

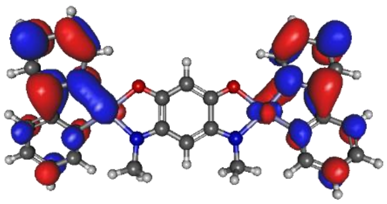

(LUMO+1) -1.7864 eV

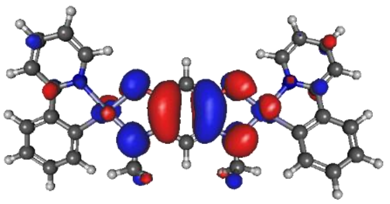

(LUMO) -2.5058 eV

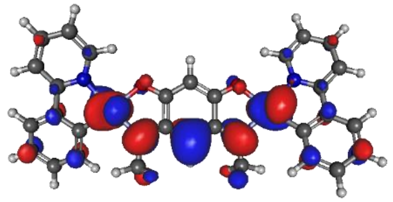

(HOMO) -4.772 eV

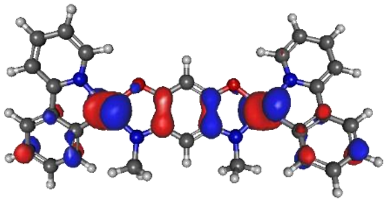

(HOMO-1) -5.3671 eV

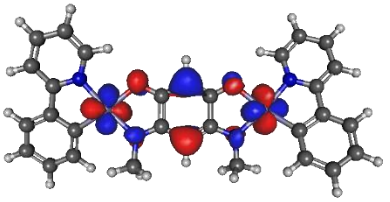

(HOMO-2) -5.575 eV

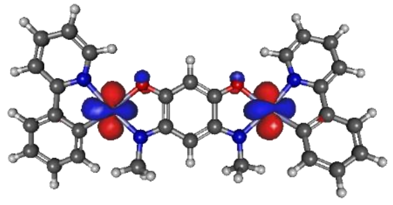

(HOMO-3) -5.6335 eV

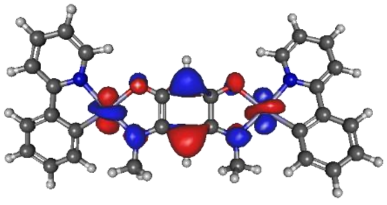

(HOMO-4) -5.7081 eV

**Figure S4:** Calculated frontier orbitals for the electronic transitions observed in Fe-dinculear molecule. (a) and (b) are the α and β orbitals, respectively.

**(a)**

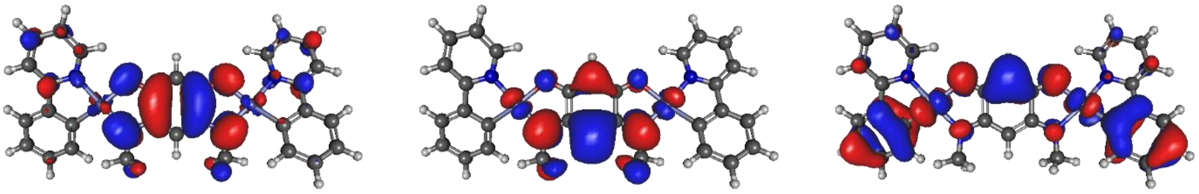

(LUMO) -2.4536 eV (HOMO) -5.1225 eV (HOMO-1) -5.7443 eV

**(b)**

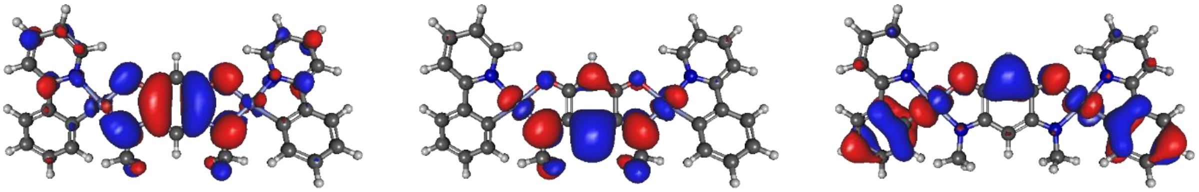

(LUMO) -2.4422 eV (HOMO) -5.0384 eV (HOMO-1) -5.5244 eV

**Figure S5:** Calculated frontier orbitals for the electronic transitions observed in Co-dinculear molecule. (a) and (b) are the α and β orbitals, respectively.

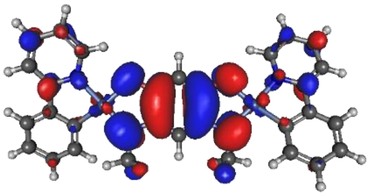

(LUMO) -2.4305 eV

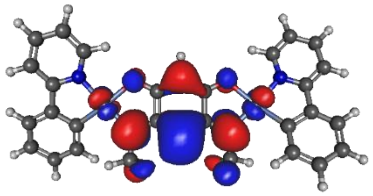

(HOMO) -5.0975 eV

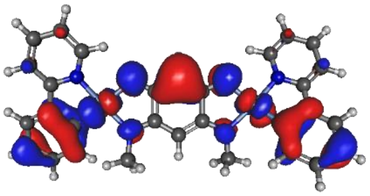

(HOMO-1) -5.6969 eV

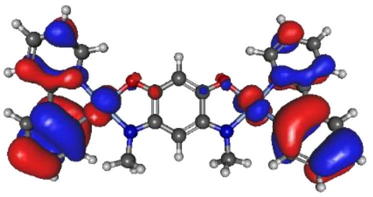

(HOMO-2) -6.0123 eV

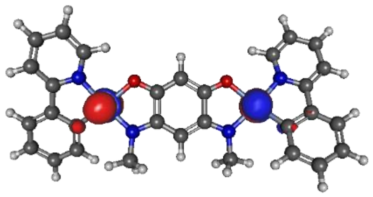

(HOMO-3) -6.0428 eV

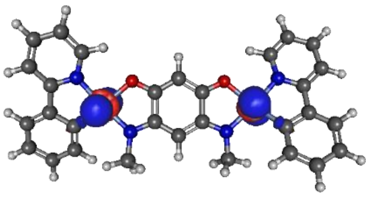

(HOMO-4) -6.0556 eV

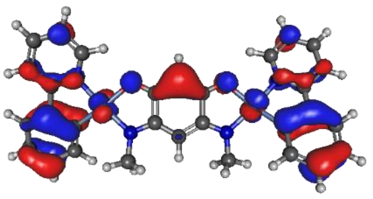

(HOMO-5) -6.2594 eV

**Figure S6:** Calculated frontier orbitals for the electronic transitions observed in Ni-dinculear molecule.

**Table S1.** Calculated magnetic moment on TM atoms in the modelled TM-dinculear molecules with different U values.

| | $Cr^{II}$-dinculear molecule | | | $Mn^{II}$-dinculear molecule | | | $Fe^{II}$-dinculear molecule | | |
|---|---|---|---|---|---|---|---|---|---|
| | Cr – 1 | Cr – 2 | Total | Mn – 1 | Mn -2 | Total | Fe - 1 | Fe -2 | Total |
| U = 0; J = 0 | 3.452 | 3.452 | 8.000 | 3.346 | 3.349 | 8.0687 | 2.065 | 2.066 | 4.0000 |
| U = 2; J = 1 | 3.562 | 3.561 | 8.000 | 3.474 | 3.474 | 8.0275 | 2.110 | 2.110 | 4.0000 |
| U = 3; J = 1 | 3.650 | 3.650 | 8.000 | 3.627 | 3.627 | 8.0007 | 2.138 | 2.139 | 4.0000 |
| U = 4; J = 1 | 3.727 | 3.727 | 8.000 | 3.867 | 3.883 | 7.9323 | 2.150 | 2.149 | 4.0000 |
| U = 5; J = 1 | 3.795 | 3.795 | 8.000 | 4.146 | 4.146 | 7.9406 | 2.142 | 2.142 | 4.0000 |
| U = 6; J = 1 | 3.853 | 3.853 | 8.000 | 4.597 | 4.597 | 10.0000 | 2.131 | 2.131 | 4.0000 |

| | $Co^{II}$-dinculear molecule | | | $Ni^{II}$-dinculear molecule | | |
|---|---|---|---|---|---|---|
| | Co – 1 | Co – 2 | Total | Ni – 1 | Ni – 2 | Total |
| U = 0; J = 0 | 1.018 | 1.015 | 2.0000 | -0.020 | -0.021 | -0.0656 |
| U = 2; J = 1 | 1.062 | 1.062 | 2.0000 | -0.017 | -0.016 | -0.0612 |
| U = 3; J = 1 | 1.080 | 1.080 | 2.0000 | -0.013 | -0.013 | -0.0589 |
| U = 4; J = 1 | 1.084 | 1.084 | 2.0000 | -0.010 | -0.010 | -0.0578 |
| U = 5; J = 1 | 1.085 | 1.085 | 2.0000 | -0.008 | -0.008 | -0.0573 |
| U = 6; J = 1 | 1.090 | 1.090 | 2.0000 | 0.006 | 0.006 | 0.0567 |

**Table S2.** The calculated TM - Ligand (in Å) in the geometry of tetra-coordinated TM for the modelled TM-dinuclear molecules.

| TM – 1 | TPSSh | GGA+U | TM – 2 | TPSSh | GGA+U |
|---|---|---|---|---|---|
| Cr - O | 2.02183 | 2.05878 | Cr - O | 2.02183 | 2.05893 |
| Cr – C | 2.09133 | 2.09802 | Cr – C | 2.09132 | 2.09815 |
| Cr – N1 | 2.04636 | 2.06087 | Cr – N1 | 2.04634 | 2.06074 |

| | | | | | |
|---|---|---|---|---|---|
| Cr – N2 | 2.07436 | 2.09565 | Cr – N2 | 2.07436 | 2.09579 |
| **Average** | **2.05847** | **2.07833** | **Average** | **2.05846** | **2.07840** |
| Mn - O | 2.04352 | 2.10480 | Mn - O | 2.04351 | 2.10456 |
| Mn – C | 2.08207 | 2.12586 | Mn – C | 2.08208 | 2.12559 |
| Mn – N1 | 2.08874 | 2.12651 | Mn – N1 | 2.08873 | 2.12632 |
| Mn – N2 | 2.17930 | 2.22890 | Mn – N2 | 2.17927 | 2.22862 |
| **Average** | **2.09841** | **2.14652** | **Average** | **2.09840** | **2.14627** |
| Fe - O | 1.94700 | 1.96550 | Fe - O | 1.94697 | 1.96538 |
| Fe – C | 1.97195 | 1.97592 | Fe – C | 1.97196 | 1.97594 |
| Fe – N1 | 1.94176 | 1.94673 | Fe – N1 | 1.94179 | 1.94665 |
| Fe – N2 | 1.96281 | 1.96709 | Fe – N2 | 1.96283 | 1.96706 |
| **Average** | **1.95588** | **1.96381** | **Average** | **1.95589** | **1.96376** |
| Co - O | 1.94681 | 1.94861 | Co - O | 1.94682 | 1.94912 |
| Co – C | 1.92657 | 1.92417 | Co – C | 1.92657 | 1.92470 |
| Co – N1 | 1.92206 | 1.91822 | Co – N1 | 1.92206 | 1.91814 |
| Co – N2 | 1.92686 | 1.92398 | Co – N2 | 1.92687 | 1.92406 |
| **Average** | **1.93057** | **1.92874** | **Average** | **1.93058** | **1.92900** |
| Ni - O | 1.92459 | 1.92998 | Ni - O | 1.92451 | 1.93002 |
| Ni – C | 1.89162 | 1.89168 | Ni – C | 1.89161 | 1.89174 |
| Ni – N1 | 1.89281 | 1.8957 | Ni – N1 | 1.89280 | 1.89571 |
| Ni – N2 | 1.89700 | 1.89540 | Ni – N2 | 1.89701 | 1.89544 |
| **Average** | **1.90151** | **1.90319** | **Average** | **1.90148** | **1.90323** |

**Table S3**. The calculated θ (O-TM-C) and Φ (N1-TM-N2) angles of the tetra-coordinated TM in the moedelled TM-dinuclear molecules.

| TM – 1 | TPSSh | GGA+U | TM – 2 | TPSSh | GGA+U |
|---|---|---|---|---|---|
| O - Cr - C | 169.0203 | 167.8013 | O - Cr - C | 169.0161 | 167.7959 |
| N1 - Cr - N2 | 168.2652 | 168.8077 | N1 - Cr - N2 | 168.2630 | 168.7966 |
| O - Mn - C | 138.2000 | 159.6974 | O - Mn - C | 138.2051 | 159.6864 |
| N1 - Mn - N2 | 115.4488 | 147.0503 | N1 - Mn - N2 | 115.4509 | 147.0680 |
| O - Fe - C | 168.7519 | 168.0782 | O - Fe - C | 168.7499 | 168.0828 |
| N1 - Fe - N2 | 169.5986 | 169.0823 | N1 - Fe - N2 | 169.5966 | 169.1007 |
| O - Co - C | 167.8093 | 167.2014 | O - Co - C | 167.8045 | 167.2276 |
| N1 - Co - N2 | 167.7488 | 168.1579 | N1 - Co - N2 | 167.7404 | 168.1927 |
| O - Ni - C | 169.0260 | 169.0090 | O - Ni - C | 169.0204 | 169.0069 |
| N1 - Ni - N2 | 168.0858 | 168.3214 | N1 - Ni - N2 | 168.0778 | 168.3138 |

**Table S4.** The electronic transitions of Cr-dinuclear molecule calculated by the TD-DFT calculations, based on the optimized structure by using B3LYP functional (The corresponding molecular orbitals are shown in Figure S3).

| Excited State | E (eV) | λ (nm) | f ( > 0.02) | Major contributions | \|CI coef\| ( > 0.3) |
|---|---|---|---|---|---|
| 2 | 2.0015 | 616.38 | 0.0947 | HOMO-1 → LUMO (α)<br>HOMO-5 → LUMO (β) | 0.7915<br>0.45201 |
| 3 | 2.12 | 584.83 | 0..0399 | HOMO → LUMO (α)<br>HOMO → LUMO (β) | 0.56547<br>0.73194 |
| 7 | 2.7029 | 458.71 | 0.1267 | HOMO-6 → LUMO (α)<br>HOMO-1 → LUMO (α)<br>HOMO-5 → LUMO (β) | 0.47407<br>0.37672<br>0.43530 |
| 10 | 2.7810 | 445.82 | 0.0446 | HOMO → LUMO+2 (α) | 0.64016 |
| 13 | 2.7810 | 445.82 | 0.0429 | HOMO-1 → LUMO+5 (α) | 0.36923 |
| 16 | 2.9030 | 427.09 | 0.0202 | HOMO-3 → LUMO+5 (α) | 0.31324 |

**Table S5.** The electronic transitions of Mn-dinuclear molecule calculated by the TD-DFT calculations, based on the optimized structure by using B3LYP functional (The corresponding molecular orbitals are shown in Figure S4).

| **Excited State** | **E (eV)** | **λ (nm)** | **f ( > 0.02)** | **Major contributions** | **\|CI coef\| ( > 0.3 )** |
|---|---|---|---|---|---|
| 2 | 2.0384 | 608.23 | 0.0704 | HOMO-1 → LUMO (α)<br>HOMO → LUMO (α)<br>HOMO-3 → LUMO (β) | 0.43020<br>0.62686<br>0.49040 |
| 3 | 2.3455 | 528.61 | 0.0231 | HOMO-1 → LUMO (α)<br>HOMO → LUMO (α)<br>HOMO → LUMO (β) | 0.67161<br>0.33505<br>0.61559 |
| 7 | 2.7801 | 476.55 | 0.0889 | HOMO-5 → LUMO (α)<br>HOMO-3 → LUMO (α)<br>HOMO-1 → LUMO (α)<br>HOMO → LUMO (α)<br>HOMO-3 → LUMO (β) | 0.47139<br>0.48550<br>0.38496<br>0.33998<br>0.47136 |
| 8 | 2.7801 | 445.97 | 0.0780 | HOMO-6 → LUMO (α)<br>HOMO-3 → LUMO (α)<br>HOMO-3 → LUMO (β) | 0.33495<br>0.76151<br>0.30443 |

**Table S6:** The electronic transitions of Fe-dinuclear molecule calculated by the TD-DFT calculations, based on the optimized structure by using B3LYP functional (The corresponding molecular orbitals are shown in Figure S5).

| **Excited State** | **E (eV)** | **λ (nm)** | **f ( > 0.02)** | **Major contributions** | **\|CI coef\| ( > 0.3 )** |
|---|---|---|---|---|---|
| 10 | 1.7713 | 699.95 | 0.1271 | HOMO-1 → LUMO (α)<br>HOMO → LUMO (α)<br>HOMO-4 → LUMO (β)<br>HOMO-2 → LUMO (β)<br>HOMO → LUMO (β) | 0.41098<br>0.46774<br>0.31882<br>0.35265<br>0.53356 |
| 16 | 2.1621 | 573.44 | 0.1275 | HOMO → LUMO (α)<br>HOMO-2 → LUMO (β) | 0.44502<br>0.69153 |
| 18 | 2.2751 | 544.96 | 0.0827 | HOMO-4 → LUMO (β)<br>HOMO-2 → LUMO (β) | 0.67873<br>0.45918 |
| 20 | 2.4089 | 514.7 | 0.0209 | HOMO-4 → LUMO (β)<br>HOMO → LUMO+2 (β) | 0.47741<br>0.61738 |
| 21 | 2.5287 | 490.31 | 0.1488 | HOMO-1 → LUMO (α)<br>HOMO-4 → LUMO (β)<br>HOMO → LUMO+2 (β) | 0.62621<br>0.33649<br>0.42590 |

**Table S7:** The electronic transitions of Co-dinuclear molecule calculated by the TD-DFT calculations, based on the optimized structure by using B3LYP functional (The corresponding molecular orbitals are shown in Figure S6).

| **Excited State** | **E (eV)** | **λ (nm)** | **f ( > 0.02)** | **Major contributions** | **\|CI coef\| ( > 0.3 )** |
|---|---|---|---|---|---|
| 15 | 2.0770 | 596.93 | 0.0798 | HOMO → LUMO (α)<br>HOMO → LUMO (β) | 0.68379<br>0.64502 |
| 17 | 2.6453 | 468.69 | 0.4268 | HOMO-1 → LUMO (α)<br>HOMO-1 → LUMO (β) | 0.58413<br>0.61066 |

**Table S8.** The electronic transitions of Ni-dinuclear molecule calculated by the TD-DFT calculations, based on the optimized structure by using B3LYP functional (The corresponding molecular orbitals are shown in Figure S7).

| Excited State | E (eV) | λ (nm) | f ( > 0.02) | Major contributions | \|CI coef\| ( > 0.3 ) |
|---|---|---|---|---|---|
| 1 | 2.0587 | 602.23 | 0.0606 | HOMO → LUMO | 0.62119 |
| 8 | 2.7877 | 444.76 | 0.4624 | HOMO-1→ LUMO | 0.58396 |
| 10 | 2.8146 | 440.50 | 0.0697 | HOMO-3 → LUMO | 0.63075 |
| 16 | 3.2393 | 982.75 | 0.1224 | HOMO-5→ LUMO | 0.61883 |

**References**

[1] Kresse G and Furthmuller J. 1996, Efficient iterative schemes for ab-initio total energy calculation using a plane-wave basis set. Phys. Rev. B 54 11169-86

[2] Perdew J P, Burke K and Ernzerhof M 1997 Generalized Gradient Approximation Made Simple [Phys. Rev. Lett. 77, 3865 (1996)] *Phys. Rev. Lett.* **78** 1396–1396

[3] Dudarev S L, Botton G A, Savrasov S Y, Humphreys C J and Sutton A P 1998 Electron-energy-loss spectra and the structural stability of nickel oxide: An LSDA+ U study *Phys. Rev. B* **57** 1505

[4] Wäckerlin C, Tarafder K, Siewert D, Girovsky J, Hählen T, Iacovita C, Kleibert A, Nolting F, Jung T A, Oppeneer P M and Ballav N 2012 On-surface coordination chemistry of planar molecular spin systems: novel magnetochemical effects induced by axial ligands *Chem. Sci.* **3** 3154–60
